# Supplementary material for: Modeling Beats and Downbeats with a Time-Frequency Transformer
Source: arXiv:2205.14701 source file (2022-05-29)
Supplement: Supplementary file 1 [file Sec6_Appendix.tex]

\section{Appendix}
\subsection{Comparison Between Three Models}

\begin{table*}[]
\begin{center}
\begin{tabular}{@{\extracolsep{\fill}}l|c|c|c}
Model & TCN & SpecTNT & SpecTNT-TCN \\
\toprule
\# Parameters      & 86,679      & 4,637,392     & 4,692,896    \\
Batch size     & 128       & 128          & 32           \\
Training time of 500 batches     & \~5.8 minutes  & \~10 minutes      & \~6.5 minutes  \\
Inference time of 100 30-sec audio clips     & \~6 seconds   & \~12.6 seconds          & \~15.1 seconds       \\

\end{tabular}
\end{center}
\caption{We trained and tested our model using 4 Tesla-V100-SXM2-32GB GPUs. Note that SpecTNT-TCN uses a batch size of 32 due to the GPU memory capacity. Theoretically it would require 4 times duration to train with the same amount of samples as SpecTNT (with a batch size of 128) does.}
\label{tab: parameters}
\end{table*}

The strength of SpecTNT is clearly its superior effectiveness for modeling downbeats, thanks to its self-attention mechanism that may help characterize longer temporal semantics. Also, the hierarchical architecture allows a smaller number of parameters compared to the regular Transformer, so it can maintain good generalization ability for MIR tasks with a smaller size of training data. However, as compared to TCN, a SpecTNT model is more complex in terms of size, so it takes longer time to process the data. Moreover, as discussed in Section 4.4, SpecTNT can suffer from the suboptimal problem in multi-task learning, i.e., SpecTNT prefers training longer which leads to better downbeat tracking performance but sacrifices some performance of beat tracking. Although, currently it is not clear about if the suboptimal problem can be fixed via weighting the loss for beats and downbeats respectively, the combination of SpecTNT and TCN can ease the problem. Detailed parameters, including training and inference time, are listed in Table~\ref{tab: parameters}.

\subsection{Qualitative and Quantitative Evaluation}
To give a quantitative explanation, the tempo and meter errors can be observed from the differences between CMLt and AMLt scores. Since AMLt counts double/half and triple/third variations as correct, larger difference between AMLt and CMLt indicates the model tends to predict the wrong tempo/meter. Moreover, our qualitative investigations indicate that SpecTNT is better at handling varying-tempo or spontaneous situations. For instance, for beat modeling in SMC, as compared to TCN, SpecTNT is successful in samples such as “SMC\_00111” (with pauses) and “SMC\_00165” (tempo varying), but unsuccessful in samples such as “SMC\_00213” where the percussive pattern is relatively complex. For downbeat cases, SpecTNT seems better at handling blues and jazz genres (e.g., “078” and “102” in Hainsworth) and loop-based songs (e.g., “236”, “157”, and “166” in Hainsworth). However, most failures happen due to phase errors, i.e., it predicts the backbeat as a beat, or it predicts the third beat in a bar as the downbeat for a 4/4 song. We will include these insights into the camera-ready version if the space permits.
